# Supplementary material for: A Grammatical Approach for Distributed Business Process Management using Structured and Cooperatively Edited Mobile Artifacts
Source: arXiv:2106.00041 source file (2021-05-31)
Supplement: Supplementary file 1 [file Appendix3.tex]

\myChapter{My thesis first: story of an improbable journey}{}\label{annexeMaThese}
\mySaveMarks

\myRestoreMarks
